# Supplementary material for: Assessing Treatment Effect Variation in Observational Studies: Results from a Data Challenge
Source: arXiv:1907.07592 source file (2019-09-13)
Supplement: Supplementary file 1 [file appendix-example.tex]

\section{Example appendix section}
\label{sec:example-theorem}

In this appendix we prove the following theorem from
Section~6.2:

%%% Local Variables:
%%% mode: latex
%%% TeX-master: "../..main"
%%% End:
